# Supplementary material for: Multi-agent Bayesian Learning with Best Response Dynamics: Convergence and Stability
Source: arXiv:2109.00719 source file (2021-09-02)
Supplement: Supplementary file 1 [file appendix_example.tex]

\section{Convergence of Best Response Dynamics in Examples 1-3}\label{apx:example}

\noindent\textbf{Example 1.} For any belief $\theta \in \Delta(\S)$, the game has a potential function 
\begin{align*}
    \Psi^{\theta}(\q)= 
\end{align*}
such that $\Psi^{\theta}(\qi, \qmi) - \Psi^{\theta}(\qi', \qmi) = \mathbb{E}_{\theta}[u_i^s(\qi, \qmi)]-\mathbb{E}_{\theta}[u_i^s(\qi', \qmi)]$ for any $\i \in \I$, and any $\qi, \qi' \in \Q$. 

Firstly, with any constant belief $\thetat=\theta$, the value of the potential function given the sequence of strategies generated by the simultaneous best response dynamics \eqref{eq:br} strictly increases. Since the value of the potential function is finite, the sequence of strategies musy converge. Thus, the simultaneous best response dynamics satisfies Assumption \ref{asu}. %This is due to the fact that the value of potential function $\Psi^{\theta}$ strictly decreases as players sequentially best responds to their opponents' strategies. 

For any $\theta \in \Delta(\S)$, and any $\qmi \in \Qmi$, the best response of player $\i$ is 
\begin{align*}
    BR_i(\theta, \qmi) = \{\}.
\end{align*}

\vspace{0.2cm}

\noindent\textbf{Example 2.} For any belief $\theta \in \Delta(\S)$, regardless of player 2's strategy, player 1's expected payoff is maximized with $\q_1=0$. Additionally, player 2's best response strategy corresponds to $\theta$ and $q_1=0$ is $\q_2 \in \{\q_2 \leq \min\{[\theta]\}\}$. Therefore, 

In step 2 of \eqref{eq:br}, $\q_1^2=0$ and $\q_2^2 \in $ three best response dynamics, the sequence of player 1's strategies converges to 0. 

\vspace{0.2cm}

\noindent\textbf{Example 3.}

\vspace{0.2cm}

\noindent\textbf{Example 4.} For any $\theta \in \Delta(\S)$, the congestion game has a potential function 
\begin{align*}
    \Psi^{\theta}(\q)= 
\end{align*}
such that $\Psi^{\theta}(\qi, \qmi) - \Psi^{\theta}(\qi', \qmi) = \mathbb{E}_{\theta}[u_i^s(\qi, \qmi)]-\mathbb{E}_{\theta}[u_i^s(\qi', \qmi)]$ for any $\i \in \I$, and any $\qi, \qi' \in \Q$.
